# Supplementary material for: Transient helix formation in semiflexible polymers without confinement effects
Source: arXiv:2002.04953 ancillary file (2020-09-17)
Supplement: Supplementary file 1 [file anc.pdf]

# SUPPLEMENTARY MATERIALS: Spontaneous helix formation in semiflexible polymers without confinement effects.

Debarshi Mitra<sup>1</sup>, Apratim Chatterji<sup>1,2\*</sup>

<sup>1</sup> Dept. of Physics, IISER-Pune, Dr. Homi Bhaba Road, Pune-411008, India.

<sup>2</sup> Center for Energy Science, IISER-Pune, Dr. Homi Bhaba Road, Pune-411008, India.

(Dated: February 10, 2020)

Generic interactions e.g. the Coulomb or other long ranged radially symmetric repulsive interactions between monomers of bead-spring model of a semi-flexible polymer induce instabilities in a initially straight polymer chain to form long lived helical structures. This mechanism can explain the spontaneous emergence of helices in stiff (bio-)polymers as effective charge of the chain increases. The helix formation is independent of the chemistry and torsional potentials are not used. So this method can be used to synthesize helical springs at length scales of  $nm-10\mu$ .

## I. SNAPSHOTS FOR FORMATION OF HELICES UNDER THE INFLUENCE OF $U_c$

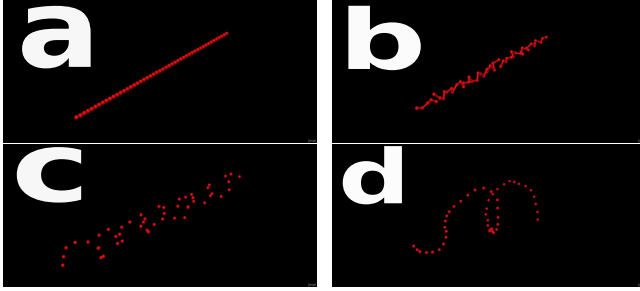

FIG. 1. Figures 1(a-d) shows various stages of the helical instability for a semi-flexible polymeric chain starting from the initial condition for case A with potential  $U_c$ . The snapshots are  $t = 0$  (b) snapshot of configuration at time  $t = 3.3 \times 10^{-4}\tau$  (c) Snapshot of the subsequent helix formed using 49 monomers at time  $t = \tau$  and (d) unwinding of the helix formed by 49 monomers at time  $t = 5\tau$ .

## II. MOVIES S1, S2, S3, S4 HELPS VISUALIZE THE INSTABILITY FOR THE 4 CASES.

Submitted along with the main and the supplementary document. The videos have been generated with the software 'VMD' and the sizes of the monomers have been increased for better visualization.

## III. HELIX FORMATION IN A POLYMER FOR DIFFERENT CHAIN LENGTHS, $N = 25$ AND $N = 100$ MONOMERS

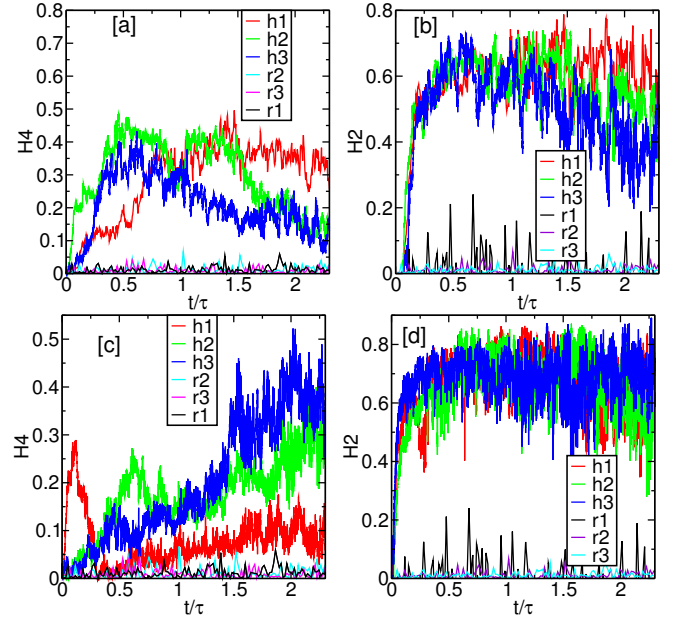

FIG. 2. Subplots (a) and (b) shows the evolution of order parameter  $H4$  and  $H2$  versus time for a semi-flexible polymer chain of 25 monomers with forces due to potential  $U_c$  between monomers. Subplots (c) and (d) shows the evolution of  $H4$  and  $H2$  versus time for a semiflexible polymer chain of 25 monomers with forces due to potential  $U_d$  between monomers.

\* apratim@iiserpune.ac.in

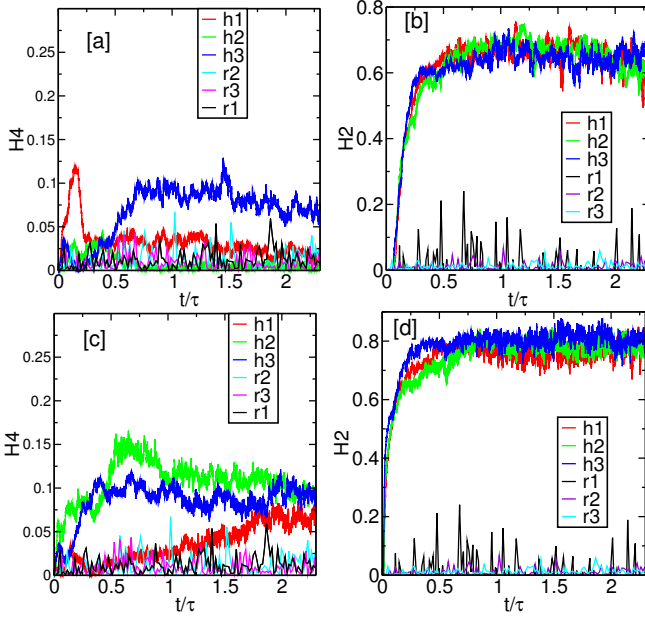

FIG. 3. Subplots (a) and (b) shows the evolution of order parameter  $H4$  and  $H2$  versus time for a polymer chain for a semi-flexible polymer chain of 100 monomers, interacting with potential  $U_c$ . Subplots (c) and (d) shows the evolution of order parameter  $H4$  and  $H2$  versus time for a semiflexible polymer chain of 100 monomers, interacting with potential  $U_d$ .

#### IV. DETAILS OF CURVED INITIAL CONDITION AT $T = 0$

We ran a simulation at temperature  $T = 0$  starting from a curved initial condition such that the  $x$  and  $z$  coordinates of the monomers are given by  $x_i = r \cos(\phi)_i$ ,  $z_i = r \sin(\phi)_i$ ,  $y_i = y_{i-1} + a$  and  $\phi_i = \phi_{i-1} + 0.1$  where  $\phi_0 = 0.7 \text{ radians}$  and  $r = 0.6$ . Note that the polymer is now curved around  $\hat{y}$  as before, as distances between monomers along  $\hat{y}$  remain unchanged. Such an initial conformation leads to helical instabilities due to forces along the  $x$  axis and the  $z$  axes and leads to the formation of helices.

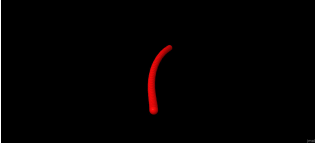

FIG. 4. Curved initial condition for a semi-flexible polymer of 49 monomers.

#### V. PROCEDURE FOR PITCH CALCULATION

To calculate the pitch of the helical structures obtained in our simulations, we calculate the dot product of the unit vectors  $\hat{r}_i$  along the chain with a vector perpendicular to the axis vector. This quantity is denoted as  $W$ . This shows periodic behaviour along the chain as is shown by Fig5(a). The Fourier transform of the same as in Fig5(b) gives us one or more peaks. The peak with the highest amplitude is termed the pitch of the helix.

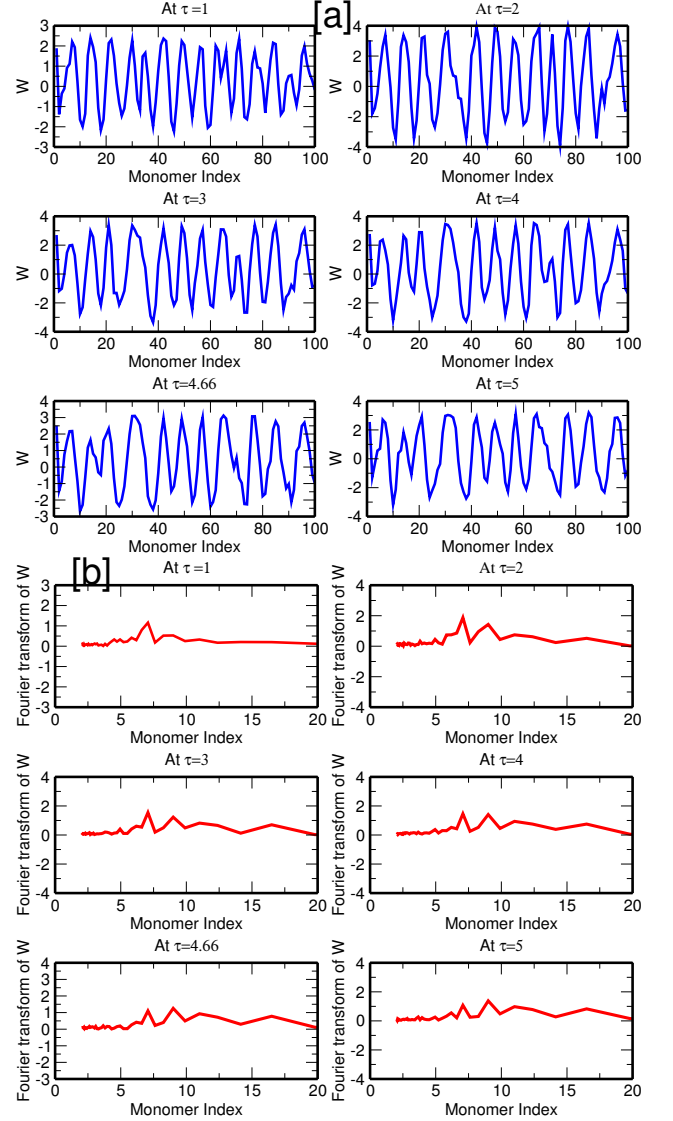

FIG. 5. Fig5(a) shows the plot of  $W$  with respect to the monomer index for given times, corresponding to chain of length 100 under the influence of  $U_c$ . Fig5(b) shows the Plot of the Fourier transform of  $W$  with respect to the monomer index for given times, corresponding to chain of length 100 under the influence of  $U_c$ .

# VI. CHANGE OF PITCH WITH RESPECT TO TIME AND SEMI-FLEXIBILITY UNDER THE INFLUENCE OF $U_d$

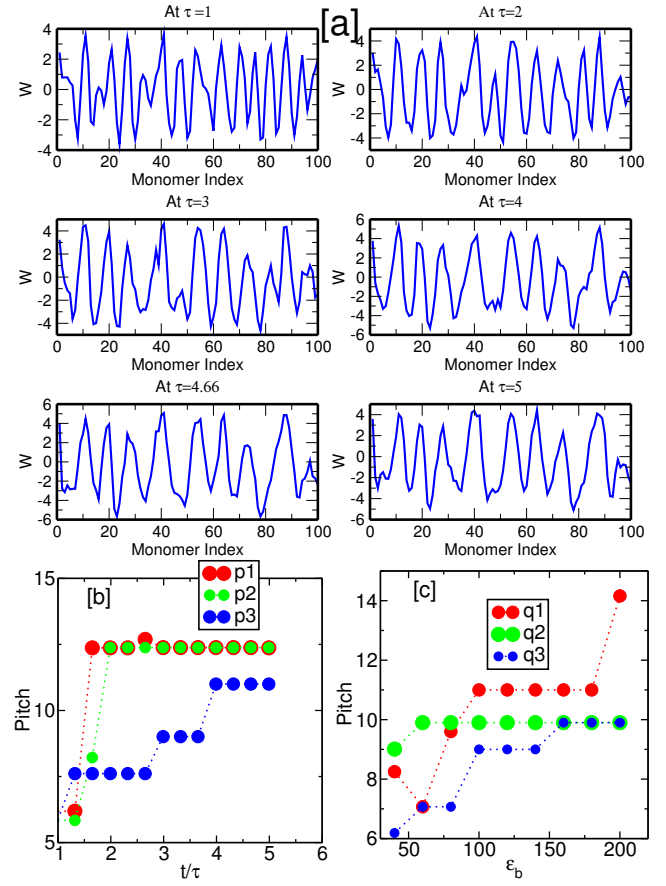

FIG. 6. Investigating how pitch changes over time and for various values of  $U_b$  under the influence of  $U_d$  (a) Plot of  $W$  with respect to the monomer index for given times, corresponding to a chain of length 100 under the influence of  $U_d$  (b) Plot of the pitch with respect to time for a chain of 100 monomers and for  $U_b = 100k_B T$  for 3 independent runs, p1, p2 and p3 keeping other parameters same as before (c) Plot of the pitch with respect to various values of  $\epsilon_b$  keeping other parameters same as before, for 3 independent runs q1, q2 and q3. The value of the pitch is calculated at time  $\tau$
